# Supplementary material for: Simulating real-time molecular electron dynamics efficiently using the time-dependent density matrix renormalization group
Source: arXiv:2409.05959 ancillary file (2024-11-13)
Supplement: Supplementary file 1 [file SI.pdf]

# Supporting Information for *Simulating real-time molecular electron dynamics efficiently using the time-dependent density matrix renormalization group*

Imam S. Wahyutama and Henrik R. Larsson

*Department of Chemistry and Biochemistry, University of California, Merced, CA 95343, USA*

October 30, 2024

## S1 Geometries

The atomic coordinates of the molecules in this work are obtained by optimizing the geometry of the corresponding molecule at a density functional theory (DFT) level using the NWCHEM quantum chemistry package.[1] The exchange-correlation functional as well as the basis set for each of the molecules are shown in Table S1. The optimized geometries for chloroacetylene, furan, acetylene, and furfural are given in Table S2, Table S3, Table S4, and Table S5, respectively.

## S2 Time propagation methods

### S2.1 Convergence of the time step targeting and time-dependent variational principle methods with respect to bond dimension and time step

In the main text, the time step targeting (TST) method does not converge smoothly in chloroacetylene both in terms of bond dimension and time step. Here, we present the same convergence study in acetylene. For all simulations in acetylene, the initial state is obtained by removing an electron from the Hartree-Fock (HF) HOMO-1 belonging to an $a_g$ symmetry of the $D_{2h}$ point group from the ground state of the neutral molecule. Therefore, the dynamics possesses an inversion symmetry at the middle of the molecular axis. We will also use the Löwdin partial charge at either of the carbons to characterize convergence. Unless otherwise stated, for all acetylene results, we use canonical HF orbitals calculated using the 6-31G[6,7] basis, an active full configuration interaction (FCI) space of CAS($20o, 9e$) with orbitals ordered by a genetic algorithm, and the state-averaged (SA) complex matrix product state (MPS) type.

The bond dimension convergence is shown in Fig. S1. Unlike chloroacetylene, in acetylene using TST, we can reach convergence with respect to the bond dimension to get a charge curve that agrees with the time-dependent variational principle (TDVP) result. However, we can also see the same trend as in choloracetylene in the main text, namely that TDVP converges faster with respect to the bond dimension than TST. For instance, the $D = 200$ curve in Fig. S1(a) can

Table S1: DFT functional and the basis set employed to calculate the optimized geometries. The last column shows the converged DFT ground state energies obtained using the corresponding optimized geometry.

| Molecule | XC functional | Basis set | Energy ($E_H$) |
|---|---|---|---|
| Chloroacetylene | B3LYP[2–4] | def2-SV(P)[5] | −536.61600774 |
| Furan | B3LYP | 6-31G | −229.95204659 |
| Acetylene | B3LYP | 6-31G | −77.26080440 |
| Furfural | B3LYP | 6-31G | −343.24086304 |

Table S2: Atomic coordinates of chloroacetylene.

| Atom | x (Å) | y (Å) | z (Å) |
|---|---|---|---|
| H | 0.000000 | 0.000000 | −2.918795 |
| C | 0.000000 | 0.000000 | −1.844234 |
| C | 0.000000 | 0.000000 | −0.633464 |
| Cl | 0.000000 | 0.000000 | 1.014353 |

Table S3: Atomic coordinates of furan.

| Atom | x (Å) | y (Å) | z (Å) |
|---|---|---|---|
| O | 0.000000 | 1.179725 | 0.000000 |
| C | 0.721833 | −0.957773 | 0.000000 |
| C | −0.721833 | −0.957773 | 0.000000 |
| C | 1.120110 | 0.347258 | 0.000000 |
| C | −1.120110 | 0.347258 | 0.000000 |
| H | 1.364650 | −1.824039 | 0.000000 |
| H | −1.364650 | −1.824039 | 0.000000 |
| H | 2.072858 | 0.845892 | 0.000000 |
| H | −2.072858 | 0.845892 | 0.000000 |

Table S4: Atomic coordinates of acetylene.

| Atom | x (Å) | y (Å) | z (Å) |
|---|---|---|---|
| H | 0.000000 | 0.000000 | −1.670620 |
| C | 0.000000 | 0.000000 | −0.605602 |
| C | 0.000000 | 0.000000 | 0.605602 |
| H | 0.000000 | 0.000000 | 1.670620 |

Table S5: Atomic coordinates of furfural.

| Atom | x (Å) | y (Å) | z (Å) |
|---|---|---|---|
| O | −0.706167 | 1.104942 | 0.000000 |
| O | 2.593148 | −0.325002 | 0.000000 |
| C | 0.255646 | 0.080432 | 0.000000 |
| C | −0.387796 | −1.137013 | 0.000000 |
| C | −1.793456 | −0.873381 | 0.000000 |
| C | −1.945022 | 0.490424 | 0.000000 |
| C | 1.644089 | 0.481704 | 0.000000 |
| H | 0.099000 | −2.099280 | 0.000000 |
| H | −2.587469 | −1.603075 | 0.000000 |
| H | −2.797325 | 1.147094 | 0.000000 |
| H | 1.812534 | 1.570275 | 0.000000 |

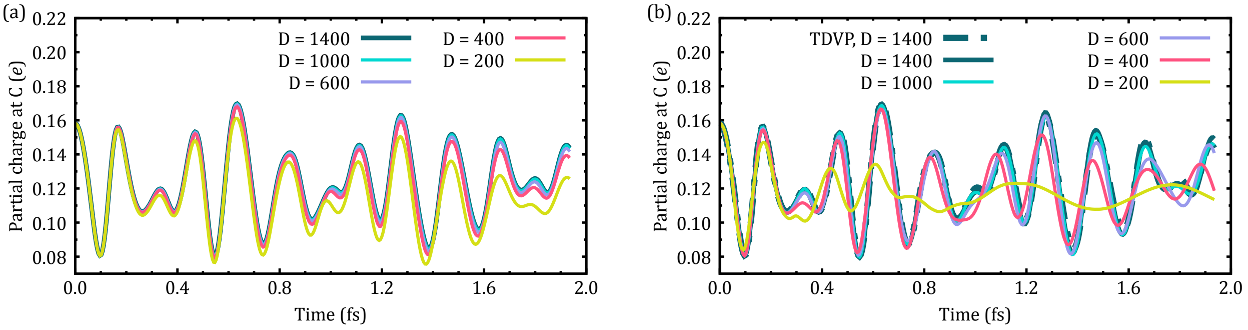


Figure S1: Convergence of the partial charge with respect to bond dimension in acetylene. $Q_{C3}(t)$ calculated using TDVP (a) and TST (b). For these simulations, we use $\Delta t = 4.84$ as and no singlet-embedding.

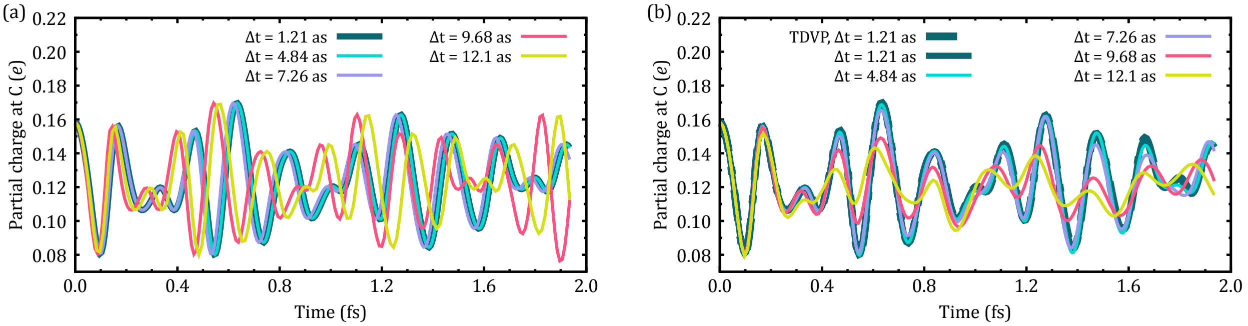


Figure S2: Convergence of the partial charge with respect to time step in acetylene. $Q_{C3}(t)$ calculated using TDVP (a) and TST (b). For these simulations, we use $D = 1000$ and no singlet-embedding.

already capture all the oscillations despite the apparent deviations in the amplitude as time passes, while the $D = 200$ curve in Fig. S1(b) becomes completely off after ∼0.25 fs.

The convergence in time step shown in Fig. S2, however, shows that TDVP and TST converge at a similar rate, with some noticeable differences in their behavior at large time steps. For TDVP (panel a), the curves at large time steps exhibit most of the oscillations in the converged curve with somewhat similar amplitudes but with some dephasing, whereas for TST (panel b) the curves at large time steps oscillate with a noticeably smaller amplitudes than the converged curve but with almost no dephasing, especially before $t = 0.95$ fs.

## S2.2 TDVP — Krylov tolerance

The forward and backward propagations of site tensors in TDVP are performed using the short iterative Lanczos method, as implemented in BLOCK2. The specific method uses a constant Krylov space size and adapts the time step based on a user-defined tolerance. The interplay between the time step and Krylov tolerance in acetylene is shown in Fig. S3. Here, we varied the tolerance for two different time steps in Fig. S3(a) and Fig. S3(b). We can see that at the shorter time step shown in Fig. S3(a), the partial charge curve with the loosest tolerance, $10^{-1}$, can already capture most of the converged oscillations. In contrast, when the time step is increased, loose Krylov tolerances will give erroneous dynamics, see Fig. S3(b). However, it quickly approaches the converged curve as the tolerance is made tighter. For instance, the curves with a tolerance of $10^{-4}$ in Fig. S3(a) and Fig. S3(b) look similar. At a tolerance of $10^{-6}$, we may consider the dynamics at both time steps to be converged.

## S2.3 TST — Sub-sweeps

Fig. 2(b) and Fig. 3(b) in the main text obtained using TST neither show smooth convergence with respect to the bond dimension nor with respect to the time step. One typical way to improve this behavior is to increase the number of

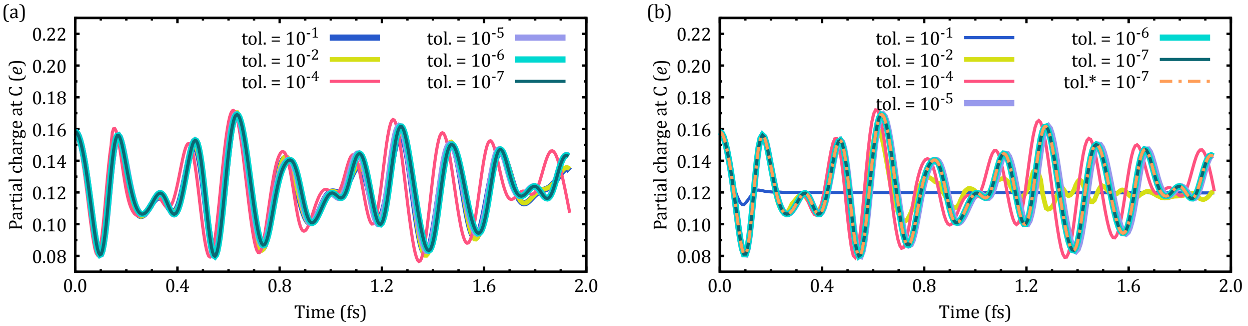


Figure S3: The effect of time step in Krylov tolerance convergence in acetylene. (a) $Q_{\mathrm{C3}}(t)$ for several Krylov tolerance values using $\Delta t = 4.84$ as and (b) $\Delta t = 7.26$ as. We use $D = 600$, a Krylov dimension of three, and singlet embedding. The curve marked as "tol.*" in panel b is the same as in panel (a) at the indicated tolerance.

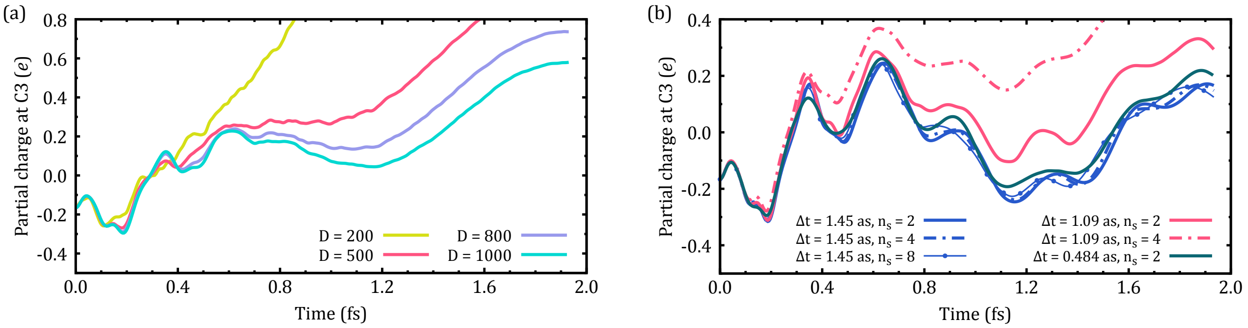


Figure S4: (a) $Q_{C3}(t)$ in chloroacetylene for several bond dimensions calculated using TST and four sub-sweeps. For comparison, all TST results in the main text, Fig. 2(b) and Fig. 3(b), are obtained with two sub-sweeps. We use $\Delta t = 0.484$ as. (b) The effect of increasing the number of sub-sweeps in $Q_{C3}(t)$ in chloroacetylene for $\Delta t = 1.09$ as and 1.45 as. The result for $\Delta t = 0.484$ as using with two sub-sweeps is shown for comparison. We use $D = 1000$, singlet embedding and a full complex MPS.

sub-sweeps within each time step. Doing this for chloroacetylene, however, does not lead to an improved convergence behavior, instead it may worsen the convergence. This is shown in Fig. S4. In Fig. S4(a), we see that the curves diverge when the number of sub-sweeps is twice as that that used in Fig. 2(b) in the main text. At other time steps, as shown in Fig. S4(b), increasing the number of sub-sweeps does not make the curve diverge, however they still do not show significant signs of convergence with respect to the number of sub-sweeps (see the $\Delta t = 1.45$ as curves).

# S3 Localized orbitals in acetylene

We demonstrated in the main text that orbital localization can speed up bond dimension convergence in time-dependent simulations, this is observed in chloroacetylene. However, this is not the case in furan, as has been shown in the main text, and also in acetylene, as will be shown below. The bond dimension scans using delocalized canonical HF orbitals and their split-localized version are shown in Fig. S5(a) and Fig. S5(b), respectively. The splitting is done by using 5 occupied and 15 unoccupied HF orbitals. As in furan in the main text, we see that the convergence of bond dimension is slower if the orbitals are localized. The ground state energies of acetylene cation as a function of bond dimension using the same orbitals as in Fig. S5 are shown in Fig. S6. Unlike the ground state energies of the furan cation in Fig. 8 of the main text, here we see that localized orbitals also do not speed up bond dimension convergence in ground state calculations, indicating that acetylene is too small for localization to be useful. Despite this differing behavior for the ground state optimization, we see that the effect of localized orbitals in bond dimension convergence for time-dependent simulations is not straightforward.

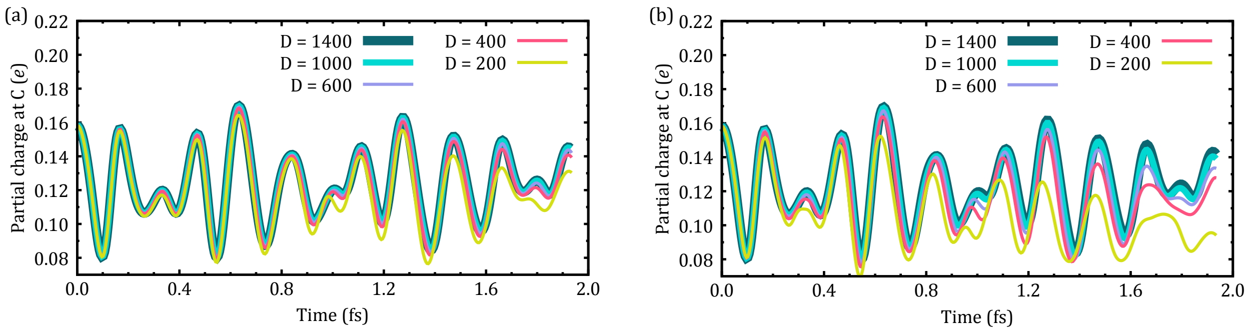


Figure S5: The effect of orbital localization in bond dimension convergence in acetylene. (a) $Q_{C3}(t)$ using delocalized canonical HF orbitals and (b) HF-based split-localized orbitals. For these simulations, we use $\Delta t = 4.84$ as, singlet embedding and a full complex MPS.

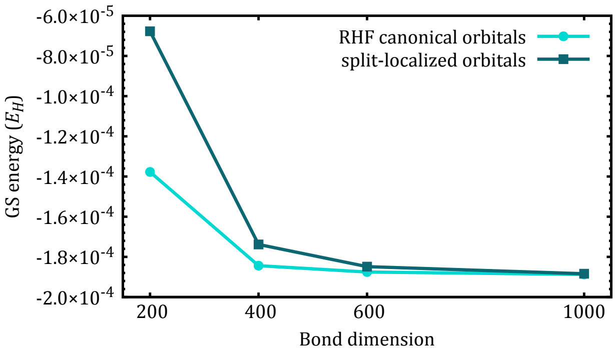


Figure S6: Ground state energy of the acetylene cation as a function of bond dimension obtained using either HF canonical orbitals (points) or split-localized orbitals (squares). These are the same orbitals employed in Fig. S5. The energies are shifted up by 76.5932 $E_H$.

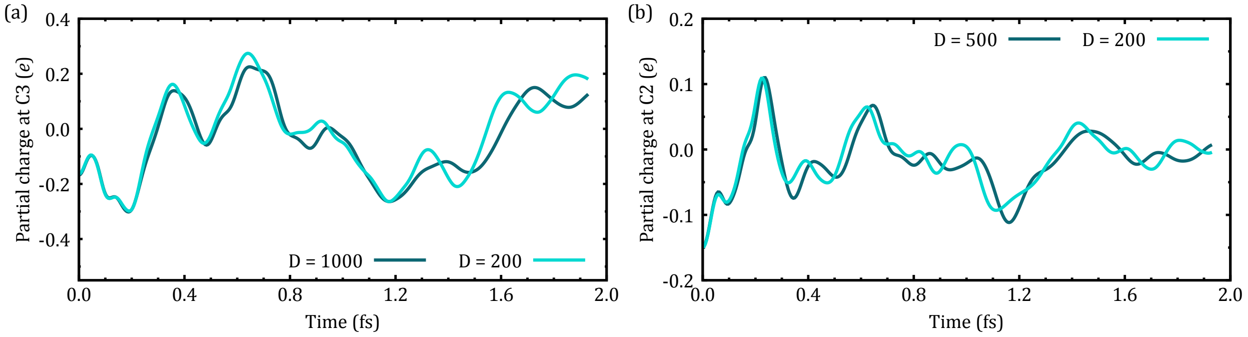


Figure S7: The dynamics produced by the preliminary MPS-FCI simulations needed for the dynamics-adapted orbitals compared to the result with the same active space but larger $D$. (a) $Q_{\mathrm{C3}}(t)$ in chloroacetylene. (b) $Q_{\mathrm{C2}}(t)$ in furan. The $D = 200$ curves in (a) and (b) correspond to the preliminary TDDMRG simulation. In (a), the active space is CAS($41o, 15e$), while in (b), it is CAS($48o, 25e$). For both simulations, we use $\Delta t = 0.968$ as, singlet embedding, and a full complex MPS.

# S4 Choice of orbitals

## S4.1 Qualitative accuracy of the preliminary run in the computation of dynamics-adapted orbitals

The preliminary run required in the first step of the computation of the density matrix (DM-) and hole-DM-adapted orbitals should be done using, whenever possible, all the available active orbitals, but with a sufficiently small bond dimension to keep the computational time reasonably low relative to the actual time-dependent density matrix renormalization group (TDDMRG) simulation that employs a smaller active space. This, however, raises the question whether the preliminary run could still capture the main characteristics of the desired dynamics. Here, we will show that this is true for the dynamics-adapted orbitals employed for chloroacetylene and furan simulations in the main text. Fig. S7 shows the partial charge resulting from the preliminary simulations used in the calculation of the dynamics-adapted orbitals in chloroacetylene and furan. In each case, we also plot a larger-$D$ result for reference, which is referred to as “MPS-FCI” in the main text. Here, we see that the chosen bond dimensions for the preliminary simulations still allow dynamics that roughly captures the one obtained at the FCI limit with a large bond dimension. Notably, however, the results from the main text in Fig. 9(c) with a reduced active space (but larger bond dimension) are closer to the large-$D$ FCI curve than the $D = 200$ preliminary curve.

## S4.2 Active space convergence

In addition to the hole-DM- and DM-adapted orbitals introduced in the main text, we also perform studies of active space convergence using three other types of orbitals. These are the ground state (GS) DMRG self-consistent field (DMRGSCF) orbitals of the neutral, GS DMRGSCF orbitals of the cation, and the state-average (SA) DMRGSCF orbitals of the cation. Next to the GS orbitals of the neutral, we investigated the SA DMRGSCF orbitals of the cation because they are optimized to describe the ground state and several excited states, which is in line with the dynamics, as it occurs in the cation where several excited states must be excited during the evolution, albeit many more excited states will be dominant than those used for the SA procedure. For the SA DMRGSCF procedure, we optimize six many-electron eigenstates.

These DMRGSCF orbitals are obtained using a bond dimension of 500. The target wave function symmetry for the neutral orbitals is $a_1$ of the $C_{2v}$ point group, while for the two cation orbitals, it is $b_1$. As initial DMRGSCF guess, we use split-localized MP2 natural orbitals (with an occupancy threshold of 0.1) of the charge state of interest (i.e., neutral or cation molecule) ordered based on their spatial locality. The DMRGSCF procedure uses an energy convergence threshold of $\Delta E = 10^{-5}\ E_H$. After convergence, the orbitals are split-localized again with an occupancy threshold of 0.3.

The active space convergence study of these three orbital types are shown in Fig. S8. To compare the performance of the five orbital types studied in this work, we plot the results using CAS($30o, 15e$) as well as the MPS-FCI result in

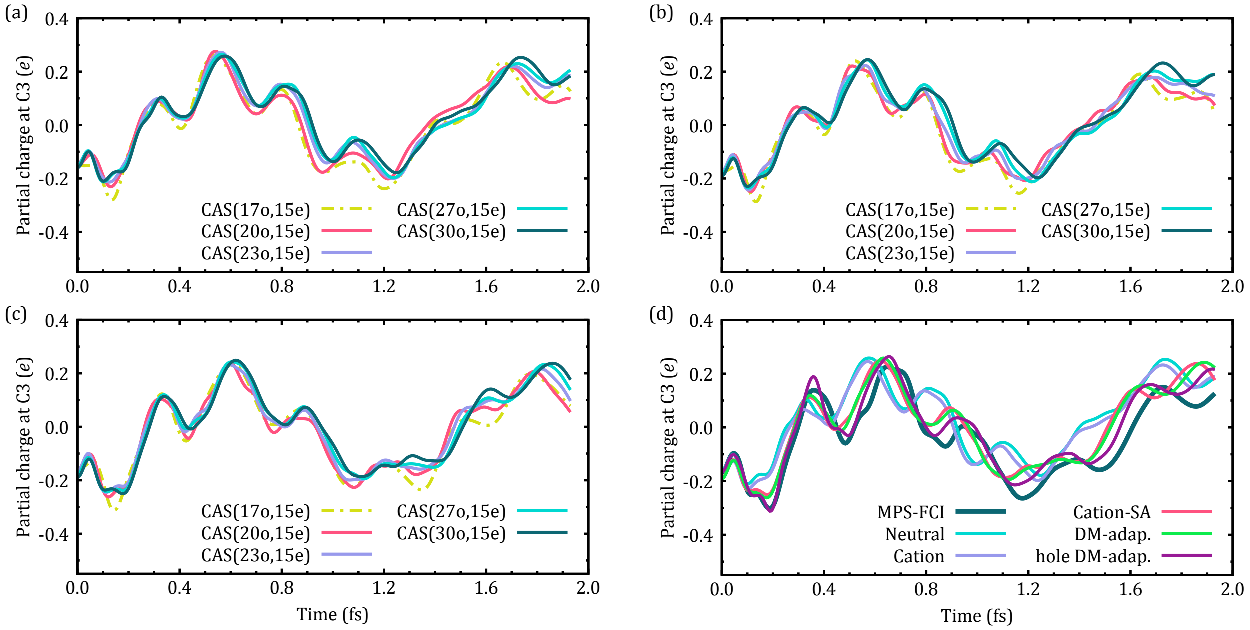


Figure S8: $Q_{C3}(t)$ in chloroacetylene obtained using several active spaces composed of (a) GS DMRGSCF orbitals of the neutral, (b) GS DMRGSCF orbitals of the cation, and (c) SA DMRGSCF orbitals of the cation. (d) A comparison of the CAS($30o, 15e$) results from panel (a), (b), (c), and the DM- as well as hole-DM-adapted orbital results from the main text together the MPS-FCI reference, whose active space is CAS($41o, 15e$). The bond dimension is 1000, $\Delta t = 0.968$ as, and the MPS is of SA complex type.

Fig. S8(d). We can see that the two GS-optimizing orbitals (denoted as "Neutral" and "Cation") are the least accurate in comparison to MPS-FCI, in fact, the two GS orbital results look very similar. The SA DMRGSCF orbital result (marked as "Cation-SA"), on the other hand, looks very similar to the DM-adapted one up to ∼1.6 fs. The hole-DM-adapted orbitals produce the closest curve to the MPS-FCI result.

# S5 Ultrafast dynamics in furfural

## S5.1 Convergence analysis

In the present section, we analyze the convergence behavior of the results presented in Section V of the main text. Fig. S9 shows that the chosen bond dimension in the main text ($D = 700$) falls within the convergence region for dipole moment components. Likewise, the chosen time steps of 0.968 as for the $\pi$ dynamics and 0.484 as for the $\sigma$ dynamics correspond to a converged time step for dipole moment component, as shown in Fig. S10. A comparison between the chosen active space size of 40 orbitals used in the main text and another one of size 45 orbitals for both initial hole symmetries, however, exhibits more non-trivial discrepancies in the form of suboscillations (Fig. S11). Nevertheless, the overall qualitative agreement between the two active spaces still is very good.

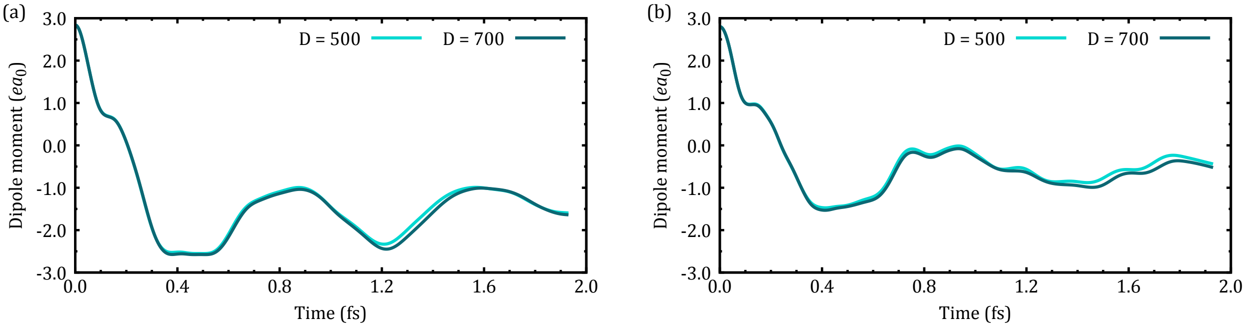


Figure S9: The bond dimension convergence in furfural. (a) The $x$ component of the dipole moment in the $\pi$ dynamics and (b) in the $\sigma$ dynamics. The simulation parameters other than the bond dimension are the same as those used in Fig. 11(c) of the main text for each type of dynamics.

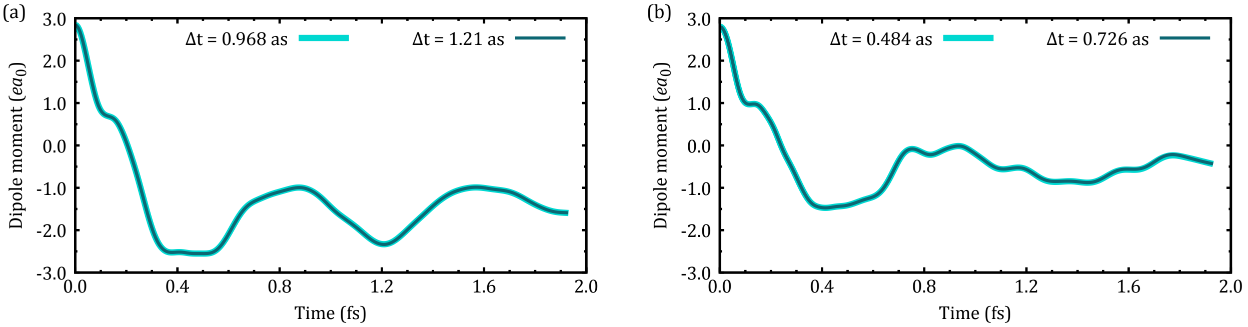


Figure S10: The time step convergence in furfural. (a) The $x$ component of the dipole moment in the $\pi$ dynamics and (b) in the $\sigma$ dynamics. The simulation parameters other than the time step are the same as those used in Fig. 11(c) of the main text for each type of dynamics, in particular, the bond dimension is 500.

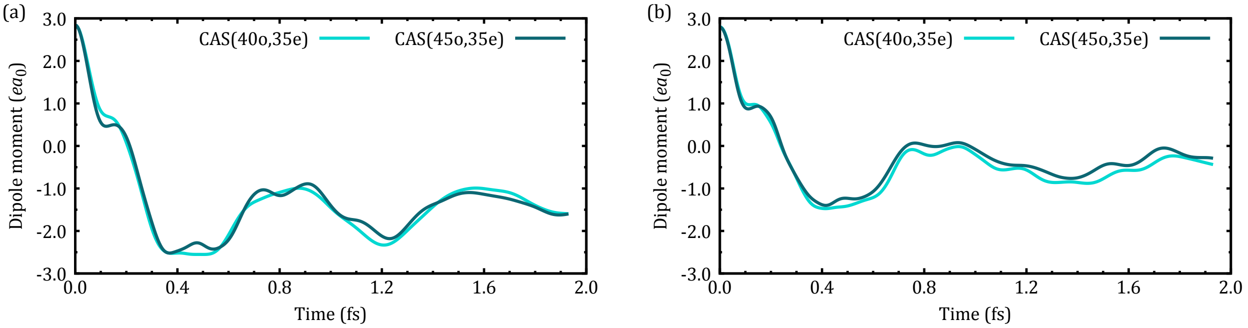


Figure S11: The active space convergence in furfural. (a) The $x$ component of the dipole moment in the $\pi$ dynamics and (b) in the $\sigma$ dynamics. The simulation parameters other than the active space size are the same as those used in Fig. 11(c) of the main text for each type of dynamics, in particular, the bond dimension is 500.

## S5.2 Analysis of hole densities

It was argued in the main text that there is a rapid shift of the dominant symmetry character of the hole in the $\sigma$ dynamics from a $\sigma$ symmetry to a $\pi$-dominant symmetry. Here, we will support this observation through an analysis of natural charge orbitals $\eta_i$, which are the eigenvectors of the hole density matrix $\mathbf{h}(t) = \boldsymbol{\rho}_0 - \boldsymbol{\rho}(t)$, at the three non-zero times at which the hole density isosurfaces are shown in Fig. 11(b) of the main text.

In terms of the natural charge orbitals, the hole density is given by

$$h(\mathbf{r}, t) = \sum_i h_i(t) |\eta_i(\mathbf{r}, t)|^2, \qquad \text{S1}$$

where $h_i$ is the hole occupancy. Fig. S12, Fig. S13, and Fig. S14 show the isosurfaces of the squared absolute values of the orbitals, $|\eta_i(\mathbf{r}, t)|^2$, of the first 20 most important natural charge orbitals at 0.484 fs, 0.968 fs, and 1.45 fs, respectively. Panel a (b) of each Figure belongs to the $\pi$ ($\sigma$) dynamics. By observing the symmetries of orbitals with large positive and large negative hole occupancies in Fig. S12(b), we do see that the $\sigma$ dynamics at 0.484 fs is already dominated by a $\pi$ character. In particular, one finds that at this time there is a significant $\pi$ hole in the cycle (with hole occupancy of 0.72) and a significant $\pi$ electron in the formyl group (with hole occupancy of −0.76). Therefore, the initial $\sigma$ hole in the formyl group has now moved into the ring and transformed into a $\pi$ hole there. Notably, the $\sigma$ dynamics at the three shown times have a moderately strong hole component whose shape is very close to that of the initial hole of the $\pi$ dynamics. For example, in Fig. S12(b), this component has a hole occupancy of 0.28.

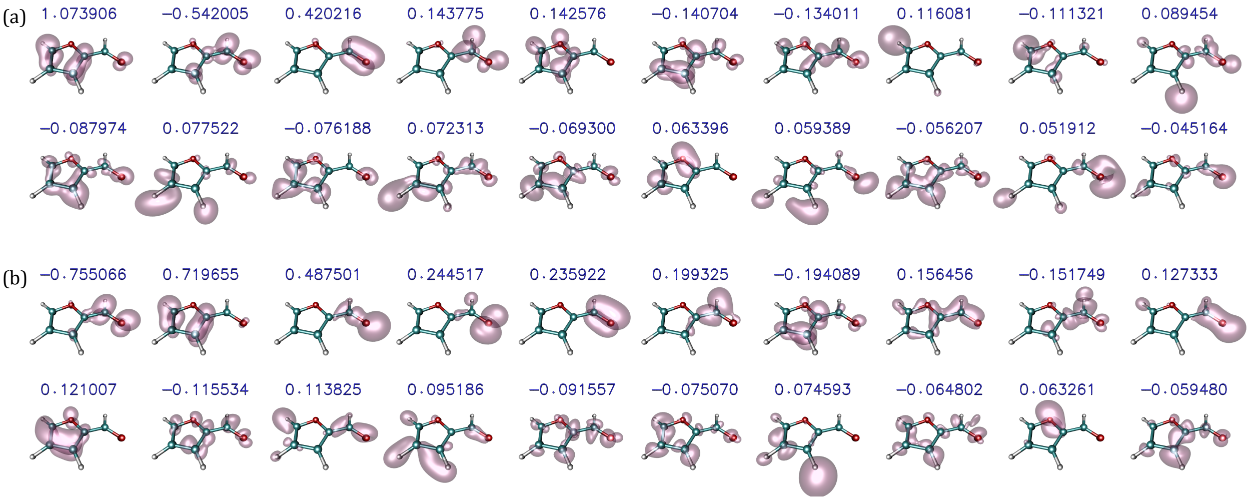


Figure S12: Squared absolute value of the first 20 natural charge orbitals with the largest magnitude of the hole occupancies in the (a) $\pi$ dynamics and (b) $\sigma$ dynamics at 0.484 fs. The isosurfaces are evaluated at $|\eta_i|^2 = 0.006$ and the number above each orbital is the corresponding hole occupancy $h_i$, with a positive (negative) value signifying a hole (electron).

# S6 Impact of state-average complex MPS type on the benchmark

In the main text, it is established that the full complex MPS leads to a more efficient simulation compared to SA complex MPS for the same bond dimension. Nevertheless, some simulations there employ the SA complex type. Here, we show that SA complex does not change the conclusion regarding the convergence behavior of the parameter being analyzed. Fig. S15 compares bond dimension convergence between TDVP (panel (a)) and TST (panel (b)). It is essentially the same as Fig. 2 in the main text except that SA complex is used. As can be seen, TDVP also facilitates a faster convergence in bond dimension than TST—the same behavior observed when full complex is used in Fig. 2 in the main text.

Fig. S16 and Fig. S17 are the SA complex equivalent of Fig. 7 and 10 (omitting panel (c)), respectively. Also in these cases, the same conclusion as the full complex counterparts in the main text can be obtained, namely, in furan: (1)

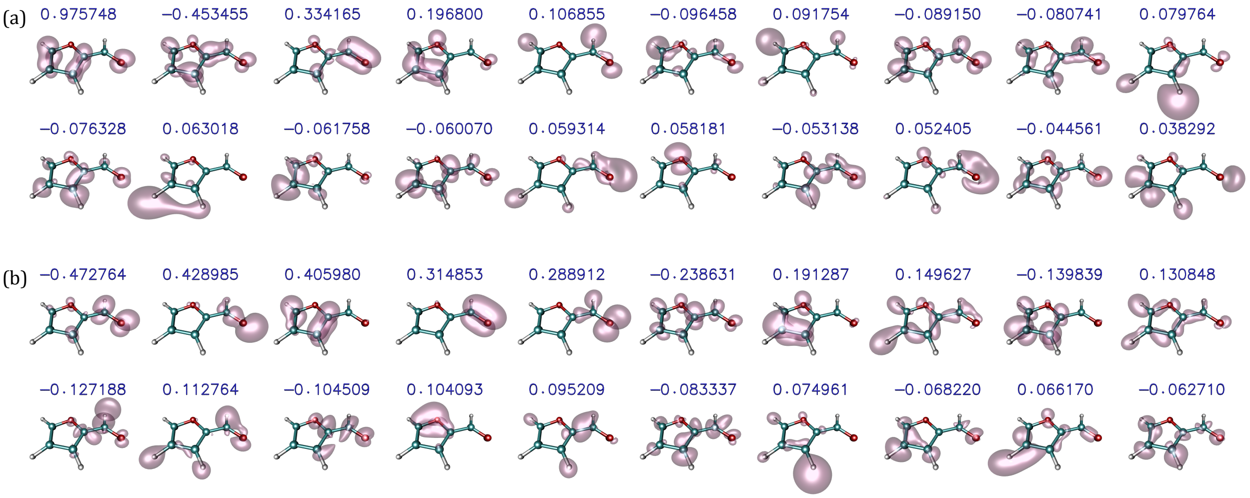


Figure S13: Squared absolute value of the first 20 natural charge orbitals with the largest magnitude of the hole occupancies in the (a) $\pi$ dynamics and (b) $\sigma$ dynamics at 0.968 fs. The isosurfaces are evaluated at $|\eta_i|^2 = 0.006$ and the number above each orbital is the corresponding hole occupancy $h_i$, with a positive (negative) value signifying a hole (electron).

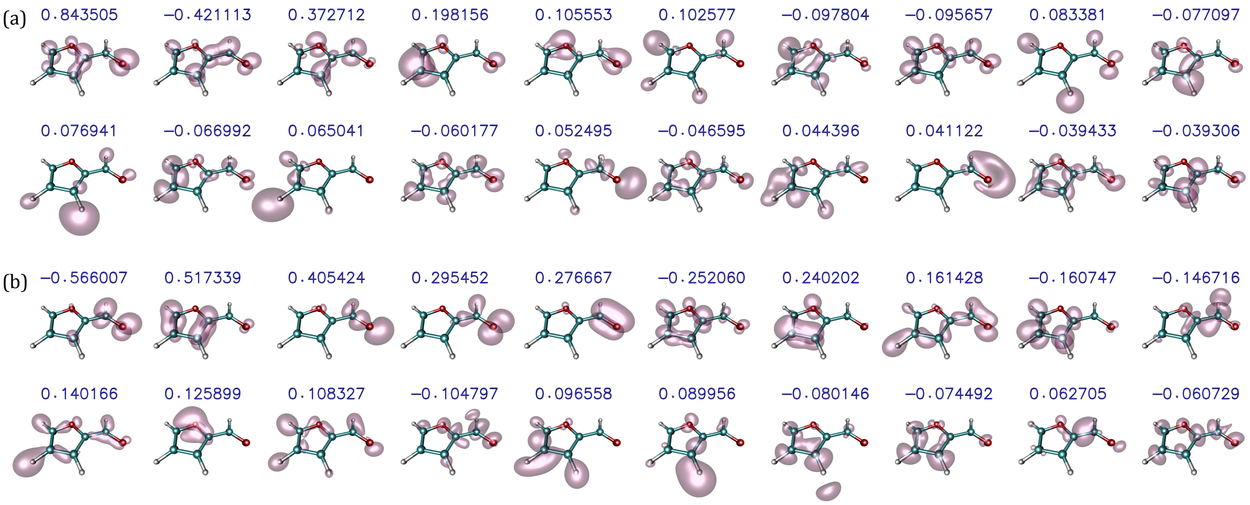


Figure S14: Squared absolute value of the first 20 natural charge orbitals with the largest magnitude of the hole occupancies in the (a) $\pi$ dynamics and (b) $\sigma$ dynamics at 1.45 fs. The isosurfaces are evaluated at $|\eta_i|^2 = 0.006$ and the number above each orbital is the corresponding hole occupancy $h_i$, with a positive (negative) value signifying a hole (electron).

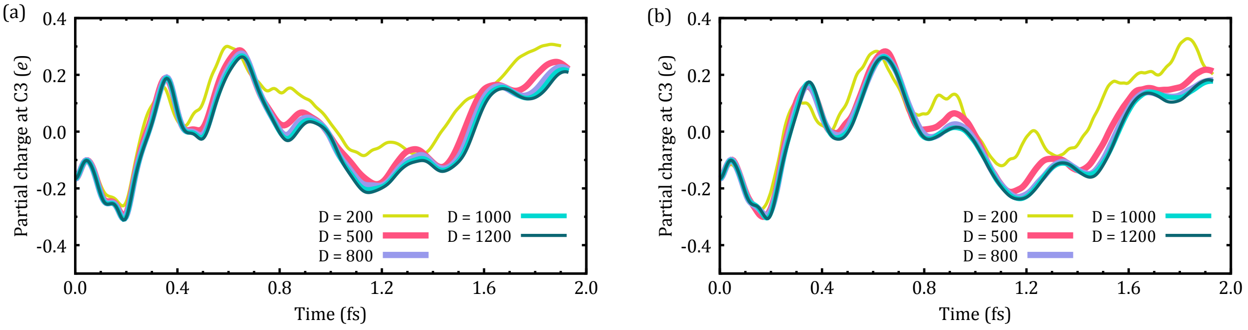


Figure S15: Partial charge around the carbon atom bonded to Cl obtained using (a) TDVP and (b) using TST for several bond dimensions. The time step is 0.484 as and the MPS is of SA complex type.

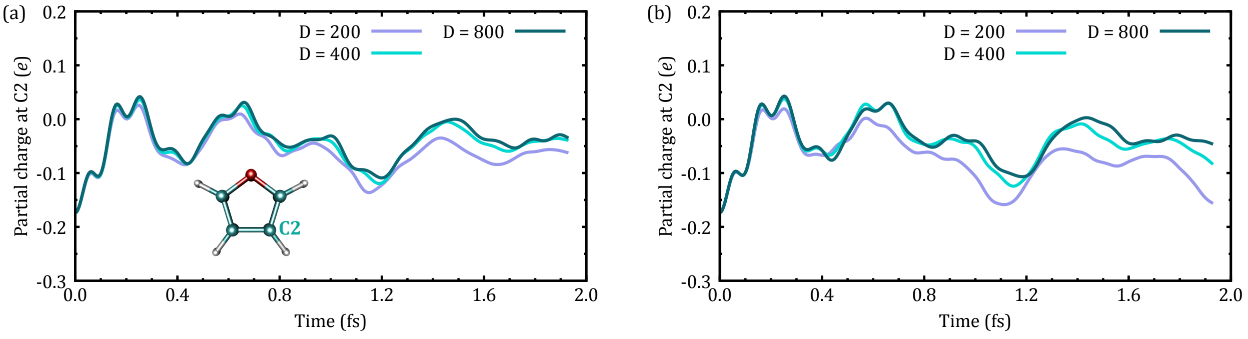


Figure S16: Partial charge around C2 of furan (see the molecule in the inset) obtained using (a) MP2 natural orbitals and (b) using localized orbitals for several bond dimensions. SA complex MPS has been used.

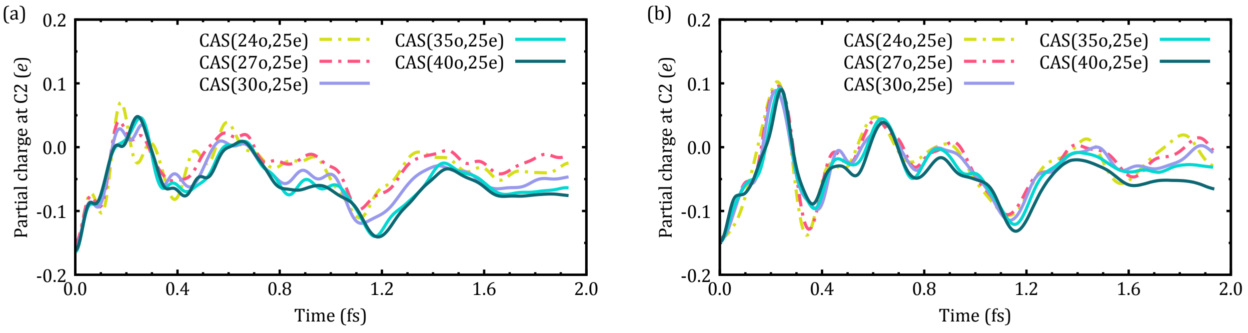


Figure S17: Partial charge around C2 of furan obtained using (a) DM-adapted orbitals and (b) using hole-DM-adapted orbitals for several active space sizes. SA complex MPS has been used.

natural orbitals (energy-localization) converge better than space-localized orbitals (Fig. S16), and (2) hole-DM-adapted orbitals converge better than DM-adapted orbitals (Fig. S17).

# References


(1) Aprà, E. et al. “NWChem: Past, present, and future”. *J. Chem. Phys.* **2020**, *152*, 184102.

(2) Becke, A. D. “Density-functional exchange-energy approximation with correct asymptotic behavior”. *Phys. Rev. A* **1988**, *38*, 3098–3100.

(3) Lee, C.; Yang, W.; Parr, R. G. “Development of the Colle-Salvetti correlation-energy formula into a functional of the electron density”. *Phys. Rev. B* **1988**, *37*, 785–789.

(4) Stephens, P. J.; Devlin, F. J.; Chabalowski, C. F.; Frisch, M. J. “Ab Initio Calculation of Vibrational Absorption and Circular Dichroism Spectra Using Density Functional Force Fields”. *J. Phys. Chem.* **1994**, *98*, 11623–11627.

(5) Weigend, F.; Ahlrichs, R. “Balanced basis sets of split valence, triple zeta valence and quadruple zeta valence quality for H to Rn: Design and assessment of accuracy”. *Phys. Chem. Chem. Phys.* **2005**, *7*, 3297–3305.

(6) Ditchfield, R.; Hehre, W. J.; Pople, J. A. “Self-Consistent Molecular-Orbital Methods. IX. An Extended Gaussian-Type Basis for Molecular-Orbital Studies of Organic Molecules”. *J. Chem. Phys.* **1971**, *54*, 724–728.

(7) Hehre, W. J.; Ditchfield, R.; Pople, J. A. “Self-Consistent Molecular Orbital Methods. XII. Further Extensions of Gaussian-Type Basis Sets for Use in Molecular Orbital Studies of Organic Molecules”. *J. Chem. Phys.* **1972**, *56*, 2257–2261.
